# Supplementary material for: Object classification on video data of meteors and meteor-like phenomena: algorithm and data
Source: arXiv:2208.14914 source file (2022-08-31)
Supplement: Supplementary file 1 [file appendix.tex]

\section{Appendix}
